# Supplementary material for: It's not a Non-Issue: Negation as a Source of Error in Machine Translation
Source: arXiv:2010.05432 source file (2020-10-12)
Supplement: Supplementary file 1 [file hyperparams.tex]

\setlength{\tabcolsep}{.07in}
\begin{tabular}{lc cccc cccc cccc}
\toprule
Test pairs &&
 \multicolumn{3}{c}{RTE}  &&
 \multicolumn{3}{c}{SNLI} &&
 \multicolumn{3}{c}{MNLI} \\
 \cmidrule(lr){3-5} \cmidrule(lr){7-9} \cmidrule(lr){11-13}
&& [1] & [2] & [3] && [1] & [2] & [3] && [1] & [2] & [3] \\
\midrule

Batch size         && 16 & 8 & 8 
                   && 32 & 32 & 32 
                   && 32 & 32 & 32 \\
Learning rate      && 2e-5 & 2e-5 & 2e-5 
                   && 1e-5 & 1e-5 & 1e-5
                   && 2e-5 & 2e-5 & 2e-5 \\
Epochs             && 10 & 50 & 50 
                   && 3 & 3 &  3
                   && 3 & 3 &  3 \\
Weight decay       && 0.0 & 0.0 & 0.0 
                   && 0.1 & 0.1 & 0.1
                   && 0.0 & 0.0 & 0.0 \\                   
\bottomrule
\end{tabular}
